# Supplementary material for: Proof Nets and the Linear Substitution Calculus
Source: arXiv:1808.03395 source file (2018-08-10)
Supplement: Supplementary file 1 [file toappendix.tex]

\gettoappendix {l:linear-subnet}
\gettoappendix {l:decomposition}
\gettoappendix {l:correct-implies-decomposable}
\gettoappendix {thm:sequentialisation}
\gettoappendix {thm:quotient}
\gettoappendix {l:context-net-plugging}
\gettoappendix {l:context-free}
\gettoappendix {thm:dynamic-isomorphism}
